# Supplementary material for: Structural Generalization in Autonomous Cyber Incident Response with Message-Passing Neural Networks and Reinforcement Learning
Source: arXiv:2407.05775 source file (2024-07-08)
Supplement: Supplementary file 1 [file appendix.tex]

\clearpage
\appendix

\section{Hyperparameters}
\label{sec:hyperparams}
\begin{tabular}{l c}
     Name & Value \\
     Global step limit & 500\,000 \\
     Environment Copies & 16 \\
     Steps per Environment & 60 \\ 
     Rollout buffer size & 1920  \\
     Minibatch size & 1920  \\
     Epochs per rollout buffer & 30 \\
     \ac{ppo} clip ratio & 0.3 \\
     Reward discount factor \(\gamma\) & 0.99 \\
     \ac{gae} \(\lambda\) & 0.95 \\
     \(C_{v}\) & 0.0001 \\
     \(C_{h}\) & 0.0 \\
     Maximum gradient L2 norm & 0.5 \\
     Learning rate & 0.0003 \\
     Activation function & \(\tanh\) \\
     \ac{gnn} embedding size & 128 \\
     \ac{mlp} embedding size & 256 \\
     \ac{mlp} layers & 2 \\
\end{tabular}

\section{Full Results}

\begin{table*}[!htpb]
\centering
\caption{Agent scores averaged over seven network variants and 1000 episodes. \ac{mpnn} models
were trained on network variant 3, a network with 13 hosts. The rows for
\ac{mlp} agents are averages of scores for six different agents, as each network variant required a separate policy.}
\begin{tabular}{lrrrrrr|r}
\toprule
Episode Length & \multicolumn{2}{c}{30} & \multicolumn{2}{c}{\textbf{50}} &
\multicolumn{2}{c}{100} & Total Score \\
Red Agent & B-Line & Meander & B-Line & \textbf{Meander} & B-Line & Meander &  \\
Model &  &  &  &  &  &  &  \\
\midrule
MPNN-G-2 & -15.13 & -5.07 & -28.75 & -11.47 & -64.01 & -30.20 & -154.63 \\
MPNN-G-3 & -15.65 & -5.25 & -48.28 & -12.54 & -160.26 & -28.27 & -270.24 \\
MPNN-G-4 & -15.80 & -6.56 & -30.43 & -14.07 & -73.42 & -32.61 & -172.90 \\
MPNN-L-2 & -14.06 & -5.14 & -25.34 & -11.11 & -53.66 & -27.65 & -136.96 \\
MPNN-L-3 & -9.86 & -4.49 & -19.25 & -9.98 & -45.42 & -24.74 & -113.75 \\
MPNN-L-4 & -13.31 & -4.90 & -27.00 & -11.19 & -64.42 & -29.27 & -150.09 \\
\midrule
Trained MLP (Ensemble) & -7.84 & -3.57 & -14.23 & -7.25 & -29.22 & -16.85 & -78.97 \\
Untrained MLP (Ensemble) & -141.23 & -45.30 & -341.05 & -170.25 & -867.80 &
-538.88 & -2104.52 \\
\bottomrule
\end{tabular}
\label{tab:variant_averages_full}

\end{table*}

\begin{table*}[!htpb]
\centering
\caption{Percentages of episodes where an agent received no negative reward, calculated over seven network variants. \ac{mpnn} models
were trained on network variant 3, a network with 13 hosts. The rows for
\ac{mlp} agents are averages for six different agents, as each network variant required a separate policy.}
\begin{tabular}{lrrrrrr|r}
\toprule
Episode Length & \multicolumn{2}{c}{30} & \multicolumn{2}{c}{\textbf{50}} &
\multicolumn{2}{c}{100} & Average \\
Red Agent & B-Line & Meander & B-Line & \textbf{Meander} & B-Line & Meander &  \\
Model &  &  &  &  &  &  &  \\
\midrule
GNN-G-2 & 1\%& 22\%& 0\%& 17\%& 0\%& 5\%& 8\% \\
GNN-G-3 & 29\%& 31\%& 22\%& 29\%& 11\%& 29\%& 25\% \\
GNN-G-4& 0\%& 5\%& 0\%& 3\%& 0\%& 0\%& 1\% \\
GNN-L-2& 0\%& 1\%& 0\%& 0\%& 0\%& 0\%& 2\% \\
GNN-L-3& 26\%& 34\%& 16\%& 18\%& 6\%& 7\%& 18\% \\
GNN-L-4& 38\%& 38\%& 35\%& 30\%& 27\%& 15\%& 31\% \\
\midrule
MLP (Ensemble) & 56\%& 28\%& 55\%& 25\%& 54\%& 19\%& 39\% \\
Untrained MLP (Ensemble) & 0\%& 0\%& 0\%& 0\%& 0\%& 0\%& 0\% \\
\bottomrule
\end{tabular}
\label{tab:variant_perfects_full}

\end{table*}

\begin{figure}[!htpb]
    \centering
    \includegraphics[width=0.45\textwidth]{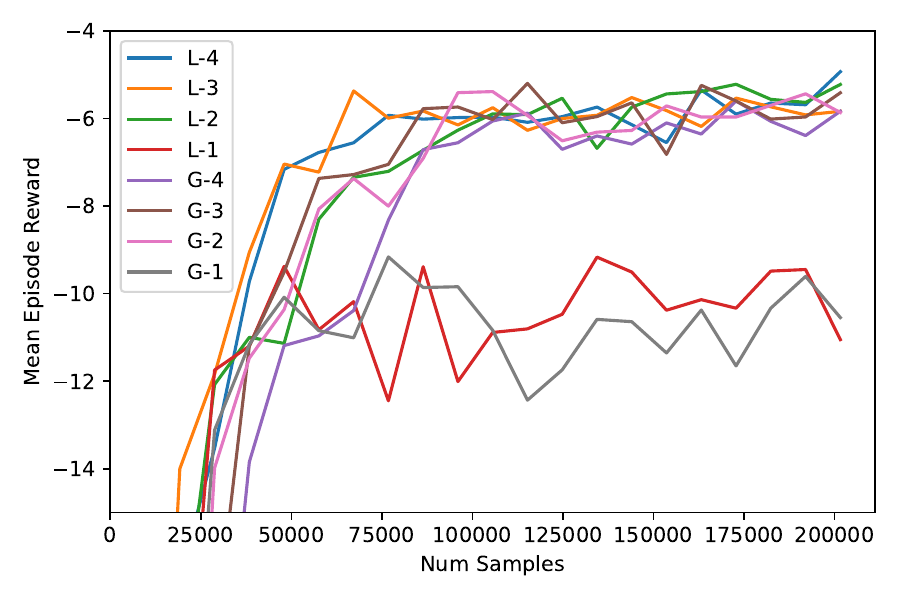}
    \caption{Reward during training for \ac{mpnn} agents with different number of layers, plotted against the total number of observations seen by the model. The most significant difference between rewards are between 1 and 2 layers.}
    \label{fig:trainreward}
\end{figure}

\section{Network Variants}

\begin{figure}[!htpb]
    \centering
    \includegraphics[width=0.45\textwidth]{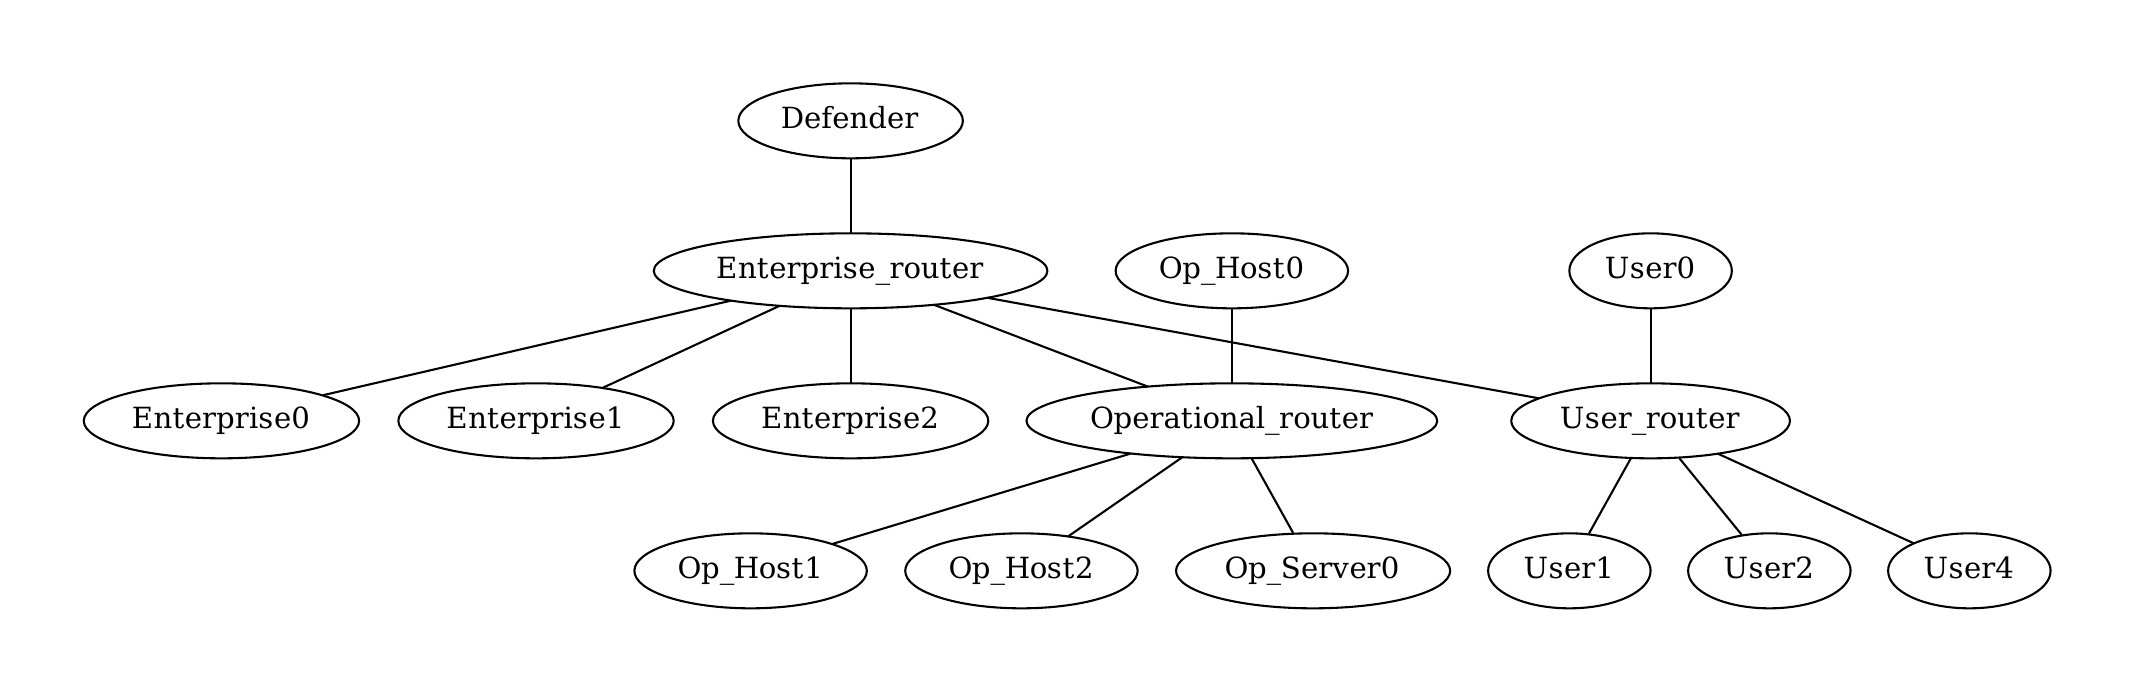}
    \caption{Variant 1. User host 3 removed.}
\end{figure}

\begin{figure}[!htpb]
    \centering
    \includegraphics[width=0.45\textwidth]{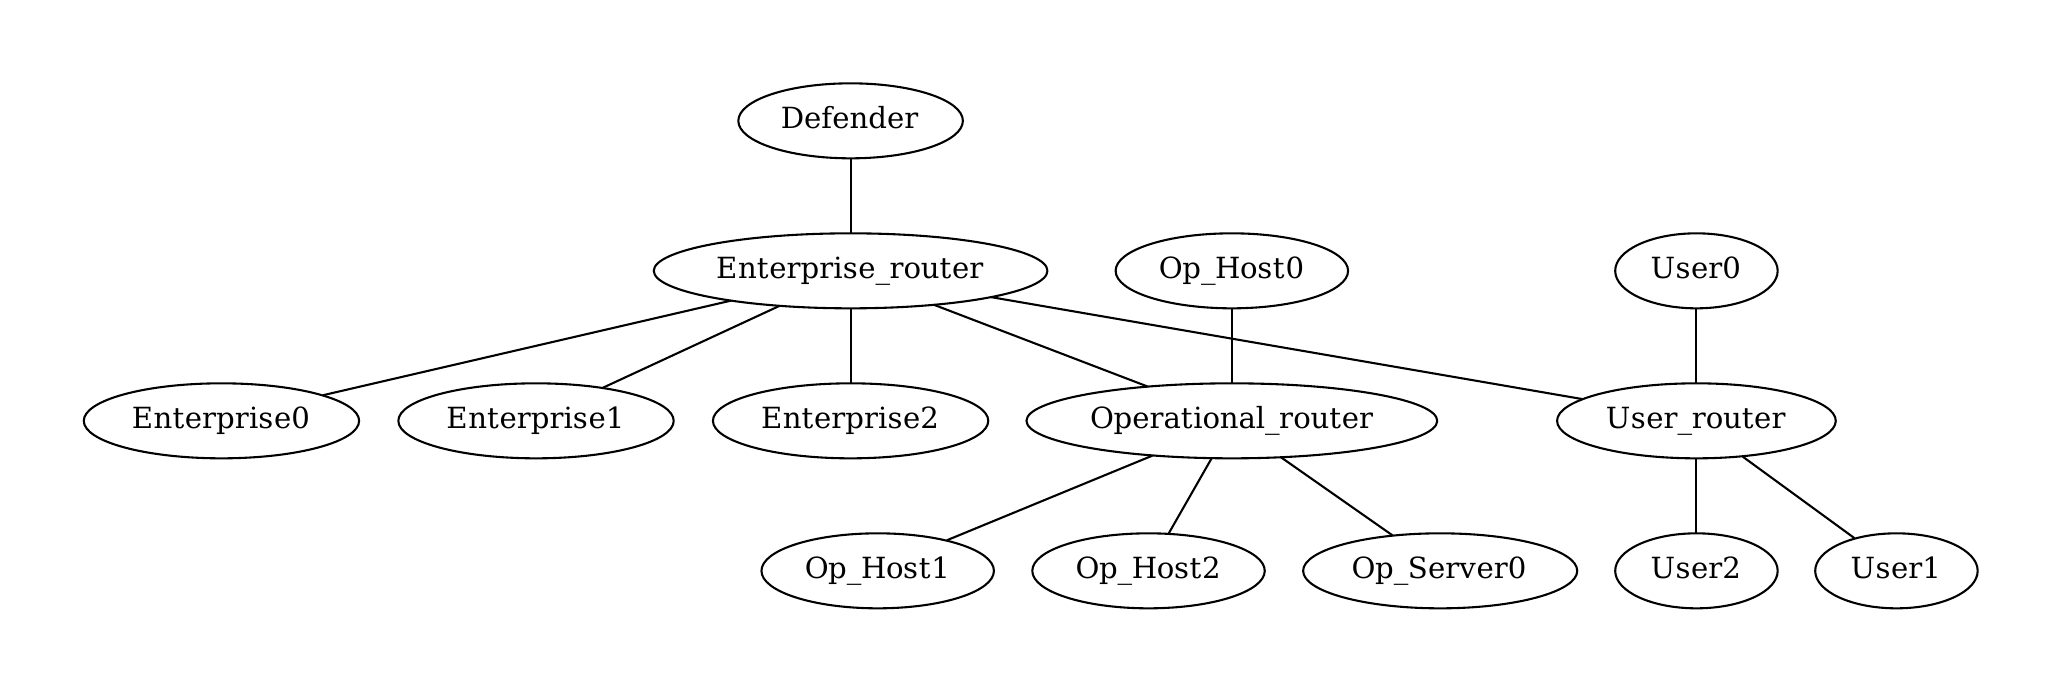}
    \caption{Variant 2. User hosts 3 and 4 removed.}
\end{figure}

\begin{figure}[!htpb]
    \centering
    \includegraphics[width=0.45\textwidth]{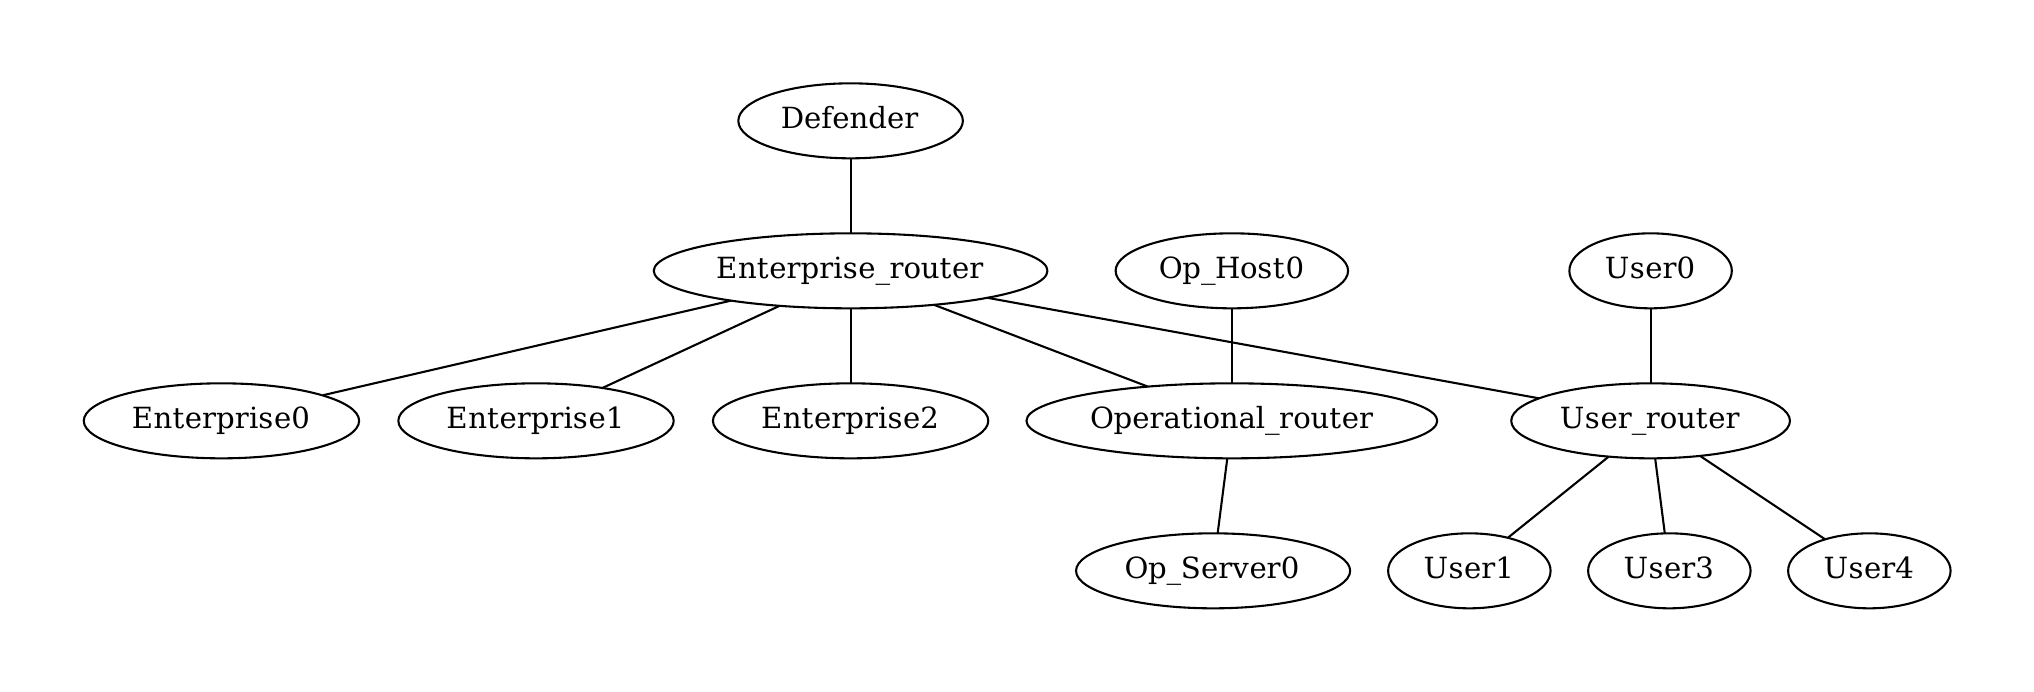}
    \caption{Variant 3. User hosts 3, 4 and Op. host 1 removed.}
\end{figure}

\begin{figure}[!htpb]
    \centering
    \includegraphics[width=0.45\textwidth]{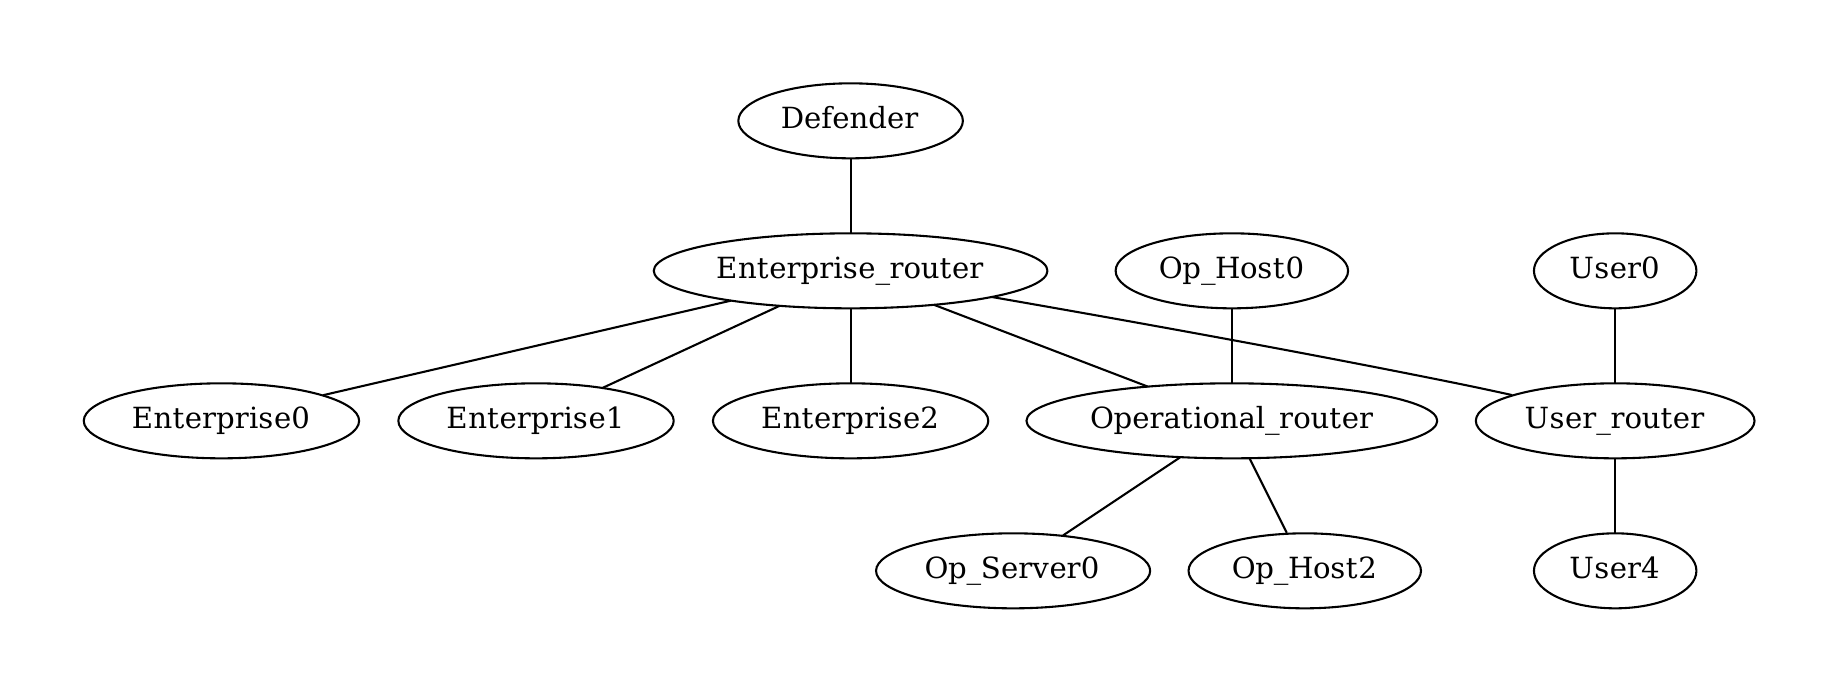}
    \caption{Variant 4. User hosts 1, 2, 3 and Op. host 1 removed.}
\end{figure}

\begin{figure}[!htpb]
    \centering
    \includegraphics[width=0.45\textwidth]{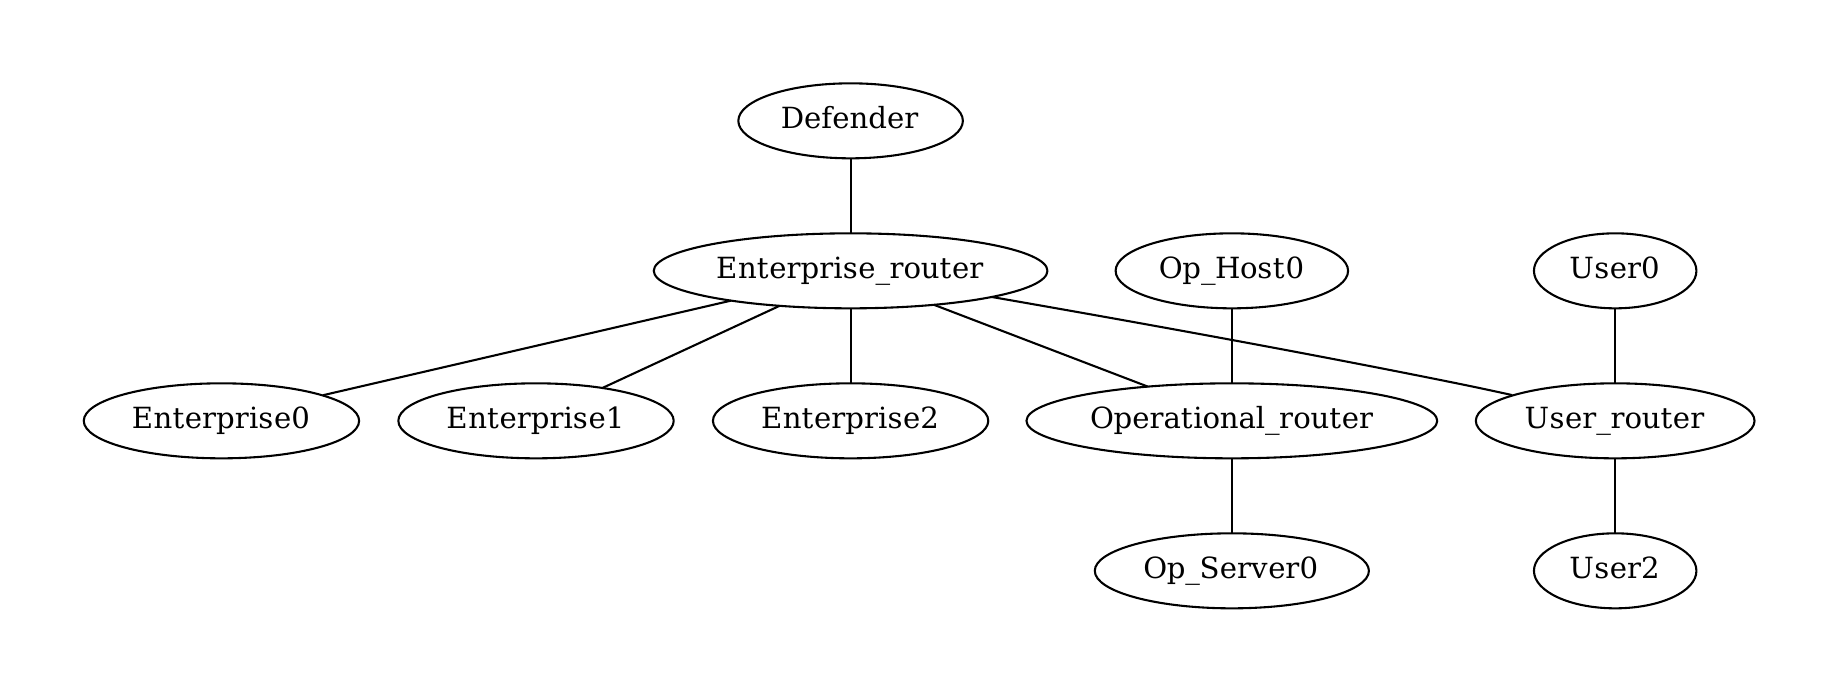}
    \caption{Variant 5. User hosts 1, 3 and 4 removed; Op. host 1 and 2 removed.}
\end{figure}

\begin{figure}[!htpb]
    \centering
    \includegraphics[width=0.45\textwidth]{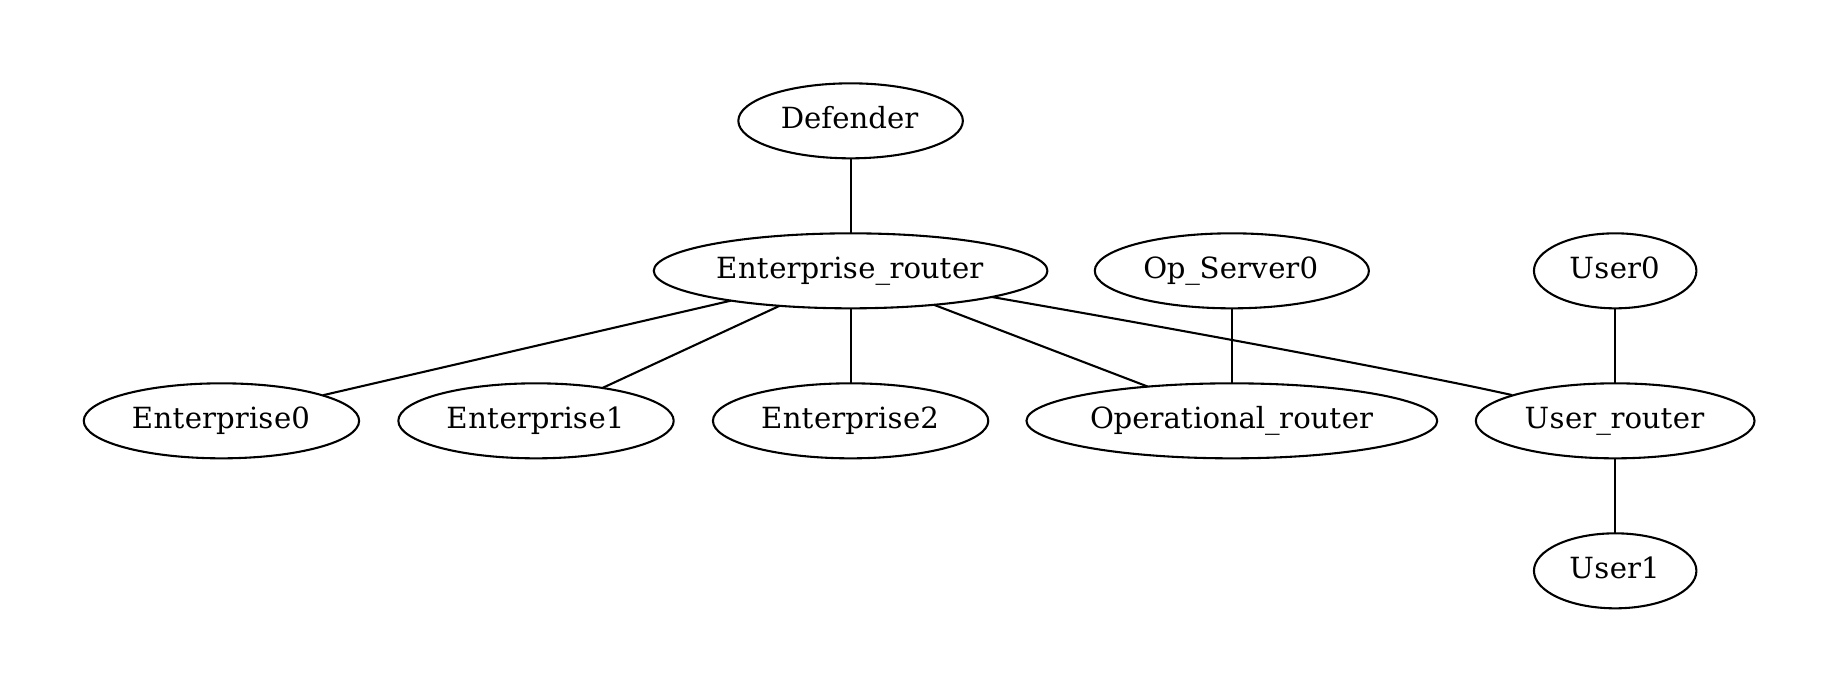}
    \caption{Variant 6. User hosts 2, 3 and 4 removed; Op. host 0, 1 and 2 removed.}
\end{figure}
